# Supplementary material for: Orbital contributions to the electron g-factor in semiconductor nanowires
Source: arXiv:1703.10091 source file (2017-06-09)
Supplement: Supplementary file 1 [file supp_mat.pdf]

# Supplemental material for
# "Orbital contributions to the electron $g$-factor in semiconductor nanowires"

Georg W. Winkler[1,*] Dániel Varjas[2], Rafal Skolasinski[2], Alexey A. Soluyanov[1,3], Matthias Troyer[1,4], and Michael Wimmer[2]

[1] *Theoretical Physics and Station Q Zurich, ETH Zurich, 8093 Zurich, Switzerland*
[2] *QuTech and Kavli Institute of Nanoscience, Delft University of Technology, 2600 GA Delft, The Netherlands*
[3] *Department of Physics, St. Petersburg State University, St. Petersburg, 199034 Russia and*
[4] *Quantum Architectures and Computation Group, Microsoft Research, Redmond WA*

(Dated: June 7, 2017)

## I. SOLVING CYLINDRICAL NANOSTRUCTURES IN THE AXIAL APPROXIMATION

### A. Numeric simulations employing the axial approximation

The cylindrical symmetry of a quantum wire allows for a considerable reduction in the computational effort of simulating the wire. To make use of this we furthermore assume that the zincblende structure itself has cylindrical symmetry by employing the so-called axial approximation [1]. In this approximation the $\mathbf{k}\cdot\mathbf{p}$-Hamiltonian has continuous rotational symmetry about the principal axis of the crystal. In this section we consider wires consisting of a zincblende semiconductor grown in the 001 direction and wurtzite semiconductor in the 0001.

In its simplest form the axial approximation amounts to equalling the two Luttinger-Kohn parameters $\gamma_2 = \gamma_3$. We choose to set $\gamma_2 = \gamma_3$ only in the terms of the Kane Hamiltonian [2] that would otherwise break the cylindrical symmetry. For the exact definition of the Hamiltonian see Tab. V in Ref. 3. The $\mathbf{k}\cdot\mathbf{p}$-parameters of InAs and InSb are taken from Ref. 4. Throughout the paper, we avoid spurious solutions by renormalizing the bare electron mass to $\gamma_0 = 5$ [5, 6].

Within the axial approximation, the wave-function can be written as [7]

$$\psi(\rho,\phi,z) = \sum_n g_n(\rho,z) e^{i l_{zn}\phi} |u_n\rangle, \tag{S1}$$

where $|u_n\rangle$ are the basis states for the 8-band $\mathbf{k}\cdot\mathbf{p}$ Hamiltonian $|j_{\text{tot}}, j_z\rangle$:

$$\begin{aligned} &|u_1\rangle = |\tfrac{1}{2}, \ \ \tfrac{1}{2}\rangle, \ |u_2\rangle = |\tfrac{1}{2}, -\tfrac{1}{2}\rangle, \ |u_3\rangle = |\tfrac{3}{2}, \ \ \tfrac{3}{2}\rangle, \ |u_4\rangle = |\tfrac{3}{2}, \ \ \tfrac{1}{2}\rangle, \\ &|u_5\rangle = |\tfrac{3}{2}, -\tfrac{1}{2}\rangle, \ |u_6\rangle = |\tfrac{3}{2}, -\tfrac{3}{2}\rangle, \ |u_7\rangle = |\tfrac{1}{2}, \ \ \tfrac{1}{2}\rangle, \ |u_8\rangle = |\tfrac{1}{2}, -\tfrac{1}{2}\rangle. \end{aligned} \tag{S2}$$

The states $|u_1\rangle$ and $|u_2\rangle$ derive from $s$-orbitals, whereas the remaining basis states are derived from $p$-orbitals. Since the Hamiltonian is block-diagonal in the total angular momentum $f_z$ one obtains the orbital part of each component $l_{zn} = f_z - j_{zn}$.

The Hamiltonian is transformed into polar coordinates $(x, y, z) \to (\rho, \phi, z)$

$$H^{\text{Polar}}_{ij}(\rho,\phi,z) = e^{-i(f_z - j_{zi})} H^{\text{Cartesian}}_{ij}(x,y,z) e^{i(f_z - j_{zj})}, \tag{S3}$$

where the $\phi$-dependece of $H^{\text{Polar}}$ drops out due to the axial approximation. The momenta $k_x$ and $k_y$ are transformed by

$$\begin{aligned} k_x &= -i\frac{\partial}{\partial x} = -i(\cos\phi\frac{\partial}{\partial\rho} - \frac{\sin\phi}{\rho}\frac{\partial}{\partial\phi}) = \cos\phi\, k_\rho - \frac{\sin\phi}{\rho} k_\phi, \\ k_y &= -i\frac{\partial}{\partial y} = -i(\sin\phi\frac{\partial}{\partial\rho} + \frac{\cos\phi}{\rho}\frac{\partial}{\partial\phi}) = \sin\phi\, k_\rho + \frac{\cos\phi}{\rho} k_\phi. \end{aligned} \tag{S4}$$

---

* winklerg@ethz.ch

Below we write all the terms that appear in the Hamiltonian and need to be transformed (note that $k_\rho$ and $k_\phi$ do not commute when the magnetic field is turned on)

$$k_+ = k_x + ik_y = e^{i\phi}(k_\rho + \frac{i}{\rho}k_\phi), \tag{S5}$$

$$k_- = k_x - ik_y = e^{-i\phi}(k_\rho - \frac{i}{\rho}k_\phi), \tag{S6}$$

$$(k_+)^2 = e^{2i\phi}[k_\rho^2 + \frac{i}{\rho}k_\rho + \frac{i}{\rho}(k_\rho k_\phi + k_\phi k_\rho) + \frac{1}{\rho^2}(-2k_\phi - k_\phi^2)], \tag{S7}$$

$$(k_-)^2 = e^{-2i\phi}[k_\rho^2 + \frac{i}{\rho}k_\rho - \frac{i}{\rho}(k_\rho k_\phi + k_\phi k_\rho) + \frac{1}{\rho^2}(2k_\phi - k_\phi^2)], \tag{S8}$$

$$k_x^2 + k_y^2 = k_\rho^2 - \frac{i}{\rho}k_\rho + \frac{1}{\rho^2}k_\phi^2. \tag{S9}$$

According to Eq. (S1), in the final matrix elements $H_{ij}$, one needs to replace each occurence of $k_\phi$ by $l_{zn} = f_z - j_{zn}$.

For a uniform magnetic field $\mathbf{B}$ in the $z$ direction the vector potential may be taken as

$$A_z = A_\rho = 0, \qquad A_\phi = \frac{1}{2}B\rho, \tag{S10}$$

which can be included in the simulation by substituting

$$k_\phi \to k_\phi - \frac{\pi}{2\phi_0}B\rho, \tag{S11}$$

where $\phi_0$ is the magnetic flux quantum.

We solve the system of coupled differential equations for the eigenmodes by rewriting it first to a generalized eigenvalue problem

$$H\mathbf{v}_n = E_n C\mathbf{v}_n, \tag{S12}$$

where $H$ is the Hamiltonian with substituted discretized expressions for the differential operators. The indices $i, j$ of $H_{ij}$ run over both the basis states Eq. (S2) and the discretized radial positions $\rho$.

We have to consider boundary conditions of both Dirichlet type $v_{ni} = 0$ and Neumann type $v_{ni} - v_{n(i+1)} = 0$. If $i$ corresponds to a position with $\rho = W$, with $W$ being the radius of the wire, the Dirichlet condition is taken. If $i$ corresponds to $\rho = 0$ the Dirichlet condition is taken for $l_z \neq 0$ and the Neumann condition for $l_z = 0$. Thus, the matrix $C_{ij}$, which encodes the boundary conditions, has only diagonal elements which are 1 if $i$ corresponds to an interior site of the wire and 0 if $i$ is either at $\rho = 0$ or $\rho = W$.

## B. Analytic estimates for the spin-orbit splitting

We calculate the spin-orbit interaction (SOI) splitting $\delta E$ of the subbands perturbatively in the rotational invariant case with $\gamma_2 = \gamma_3$ in a circular wire. We use the continuum Hamiltonian in cylindrical coordinates. Starting from the exact solution in the $\gamma_1 = \gamma_2 = \gamma_3 = 0$ case [8] we find a splitting that lowers the energy of subbands with parallel orbital and spin angular momentum using the minimal boundary amplitude condition. This splitting scales as $W^{-4}$ for thick wires and as $\Delta$ for small $\Delta$.

### 1. *Exact solution of a special case*

The real-space continuum problem can be exactly solved for the electron-like wave functions when $\gamma_1 = \gamma_2 = \gamma_3 = 0$. Following Ref. 8 we express the hole-like components in terms of the electron-like ones from the Schrödinger equation, and substitute it back to the electron component equation to get the Helmholtz-equation

$$\left\{\left[\frac{P^2}{3}\left(\frac{2}{E+E_0} + \frac{1}{E+E_0+\Delta}\right) + \frac{\gamma_0}{2m_0}\right]\nabla^2 + E\right\}\psi_{e\sigma}(\mathbf{r}) = 0 \tag{S13}$$

where $\nabla^2$ is the Laplacian, $E$ is the (unknown) energy of the state and $\psi_{e\sigma}(\mathbf{r})$ is the wave function amplitude in the electron-like bands (the equations are identical for the two spin sectors). The full wave-function, including the hole-like components can be written as

$$\psi_\uparrow(\mathbf{r}) = \begin{pmatrix} 1 & 0 & -\frac{k_- P}{\sqrt{2}(E_0+E)} & \frac{\sqrt{\frac{2}{3}} k_z P}{E_0+E} & \frac{k_+ P}{\sqrt{6}(E_0+E)} & 0 & -\frac{k_z P}{\sqrt{3}(\Delta+E_0+E)} & -\frac{k_+ P}{\sqrt{3}(\Delta+E_0+E)} \end{pmatrix} \psi_{e\uparrow}(\mathbf{r}) \tag{S14}$$

$$\psi_\downarrow(\mathbf{r}) = \begin{pmatrix} 0 & 1 & 0 & -\frac{k_- P}{\sqrt{6}(E_0+E)} & \frac{\sqrt{\frac{2}{3}} k_z P}{E_0+E} & \frac{k_+ P}{\sqrt{2}(E_0+E)} & -\frac{k_- P}{\sqrt{3}(\Delta+E_0+E)} & \frac{k_z P}{\sqrt{3}(\Delta+E_0+E)} \end{pmatrix} \psi_{e\downarrow}(\mathbf{r}) \tag{S15}$$

where for a cylindrical wire the momenta can be written in cylindrical coordinates as in Eq. (S4). The hole-like components of the real space wave-function are obtained by acting with the differential operators on the electron-like wave-function on the right.

As the equation is invariant under rotations around the $z$ axis and translations along the $z$ axis, the wave-function can be separated as $\psi_{e\uparrow}(\rho, \phi, z) = R_{l\sigma}(\rho) e^{il\phi} e^{ik_z z}$, substituting this we get the Bessel equation for the radial part

$$\left( \frac{d^2}{d\rho^2} + \frac{1}{\rho}\frac{d}{d\rho} - \frac{l^2}{\rho^2} + \chi^2 \right) R_{l\sigma}(\rho) = 0 \tag{S16}$$

with

$$\chi^2 = -k_z^2 + E \bigg/ \left[ \frac{P^2}{3} \left( \frac{2}{E+E_0} + \frac{1}{E+E_0+\Delta} \right) + \frac{\gamma_0}{2m_0} \right] \tag{S17}$$

where $\chi$ is the radial wavenumber and is determined by the boundary conditions. The solutions can be written in terms of Bessel functions $R_{l\sigma}(\rho) = J_l(\chi\rho)$. Setting $k_z = 0$, the full wave function can be written as

$$\psi_{l\uparrow}(\rho, \phi) = \begin{pmatrix} 1 & 0 & \frac{ie^{-i\phi} P (l + ik_\rho \rho)}{\sqrt{2}(E_0+E)\rho} & 0 & \frac{e^{i\phi} P (il + k_\rho \rho)}{\sqrt{6}(E_0+E)\rho} & 0 & 0 & -\frac{e^{i\phi} P (il + k_\rho \rho)}{\sqrt{3}(\Delta+E_0+E)\rho} \end{pmatrix} R_{l\uparrow}(\rho) \tag{S18}$$

$$\psi_{l\downarrow}(\rho, \phi) = \begin{pmatrix} 0 & 1 & 0 & \frac{ie^{-i\phi} P (l + ik_\rho \rho)}{\sqrt{6}(E_0+E)\rho} & 0 & \frac{e^{i\phi} P (il + k_\rho \rho)}{\sqrt{2}(E_0+E)\rho} & \frac{ie^{-i\phi} P (l + ik_\rho \rho)}{\sqrt{3}(\Delta+E_0+E)\rho} & 0 \end{pmatrix} R_{l\downarrow}(\rho) \tag{S19}$$

where we used that the action on our ansatz amounts to the replacement of $k_\phi$ with $l$. The different hole-like Bloch states have different internal angular momentum, but the total angular momentum of each component is the same, this is manifest in the extra orbital phase factors in the expression.

The hole-like contribution is proportional to the radial derivative of the wave function. As the Bessel-functions cannot have both vanishing magnitude and derivative at finite $\rho$, it is not possible to demand vanishing of all components of the wave function at the boundary. In the large wire (large $W$ and small $\chi$) limit the hole-like amplitude is suppressed, so demanding the electron-like component to vanish is approximately a good boundary condition.

### 2. *Minimal boundary amplitude boundary condition*

We assume that the system is infinite, but the states are confined by a large potential $V$ at the boundary. Assuming $V$ is much larger than any of the energy scales in the problem, then the wave function decays exponentially outside as

$$\psi(W) \approx e^{-(\rho - W)\sqrt{\frac{2m^*}{\hbar^2} V}} \tag{S20}$$

where $W$ is the radius of the wire where the potential step is. The expectation value of the potential energy goes as $\sqrt{\frac{\hbar^2}{2m^*} V} |\psi(W)|^2$, so in the large V limit the wave function amplitude is minimized, and the states get shifted up as $\sqrt{V}$.

We express the magnitude squared of the wave function on the boundary using our previous expression.

$$|\psi_{l\sigma}(W, \phi)|^2 = R^2 \left( 1 + \frac{l^2(2a+b)}{3W^2} \right) + \sigma l R R' \frac{2(a-b)}{3W^2} + (R')^2 \frac{(2a+b)}{3W^2} \tag{S21}$$

where $\sigma = \pm 1$ stands for up and down spin,

$$a = \frac{P^2}{(E_0+E)^2}, \tag{S22}$$

$$b = \frac{P^2}{(E_0+E+\Delta)^2} \tag{S23}$$

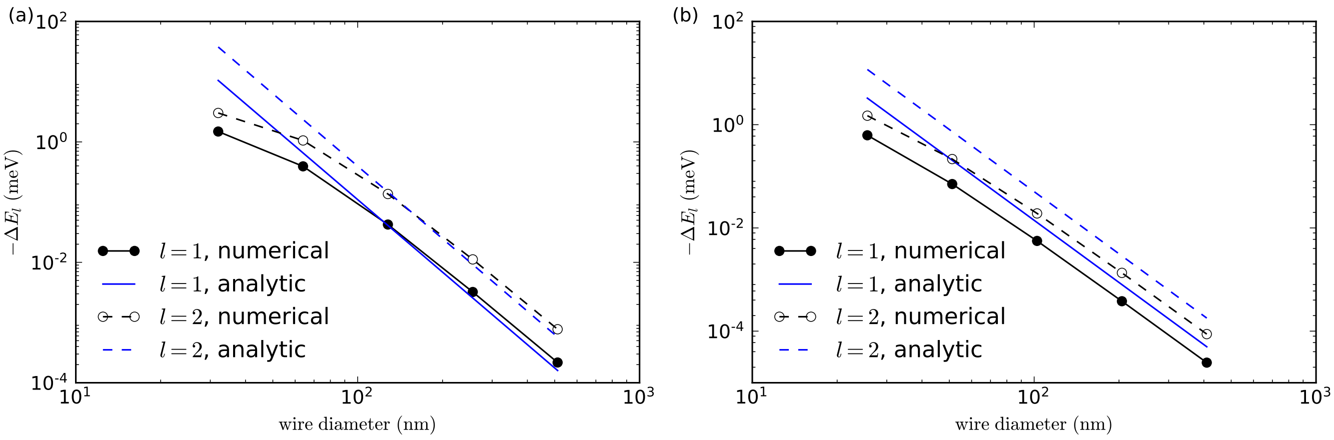


FIG. S1. (a) ((b)) Diameter dependence of the SOI splitting $\Delta E_1$ and $\Delta E_2$ for InSb (InAs) wires with soft boundary conditions. The analytic approximation of Eq. (S28) is shown for comparison.

are constants with length squared dimension and we introduced the dimensionless quantity $\chi' = \chi W$, such that $R = J_l(\chi W) = J_l(\chi')$ and $R' = W \frac{dJ_l}{d\rho}(\chi W) = \chi' J_l'(\chi')$. It can be seen that in the $W^2 \gg a$, $b$ limit (for InSb $b < a \approx 10\text{nm}^2$) the total amplitude can be minimized by minimizing the amplitude in the electron bands. This happens when $\chi' = z_{lp}$, the $p$'th root of $J_l$.

For finite $W$ we expand around this solution. To get a tractable approximation we can treat $R$ and $R'$ as independent variables and express $R$ that minimizes the amplitude in terms of $R'$:

$$R = -\sigma l R' \frac{(a-b)}{3W^2 + (2a+b)l^2}. \tag{S24}$$

The right hand side does not depend on $\gamma_0$ and is linear in $\Delta$ for small values and $E$ can be set to zero for approximate calculations if the subband energy is much smaller than the bandgap, $E \ll E_0$. We expand both sides to first order in $\delta\chi' = \chi' - z_{lp}$ and use the identity[9] $J_l'(z_{lp}) + z_{lp} J_l''(z_{lp}) = 0$ to get

$$\delta\chi' = -\sigma l z_{lp} \frac{a-b}{3W^2 + (2a+b)l^2}. \tag{S25}$$

Such a change in $\chi'$ effectively renormalizes the radius of the wire and results in a splitting between states with different total angular momentum. From Eq. (S17) the energy $E$ of a state in the small $\chi$ (large $W$, small $l$ and $p$ and small $E$) limit is approximately

$$E_{lp} = \frac{z_{lp}^2 P^2}{3W^2} \frac{3E_0 + 2\Delta}{E_0(E_0+\Delta)}. \tag{S26}$$

where we set $\chi = z_{lp}/W$ ignoring SO corrections. Note that this approximation does not depend on $\gamma_0$. Substituting $\chi'$ with $\chi' + \delta\chi'$ from (S25) and expanding to linear order the energy change induced by SOI is

$$\delta E_{lp\sigma} = -\sigma l \frac{2E_{lp}(a-b)}{3W^2 + (2a+b)l^2}. \tag{S27}$$

In the large $W$ limit the subband splitting is (dotted lines in Fig. S1)

$$E_{lp\uparrow} - E_{lp\downarrow} = -l \frac{4 z_{l,p}^2 P^4 \Delta(\Delta + 2E_0)(2\Delta + 3E_0)}{9W^4 E_0^3 (\Delta + E_0)^3}, \tag{S28}$$

which for the lowest $l = 1$ subband gives

$$E_{11\uparrow} - E_{11\downarrow} \approx -\frac{1}{W^4} 687 \text{ eV nm}^4 \tag{S29}$$

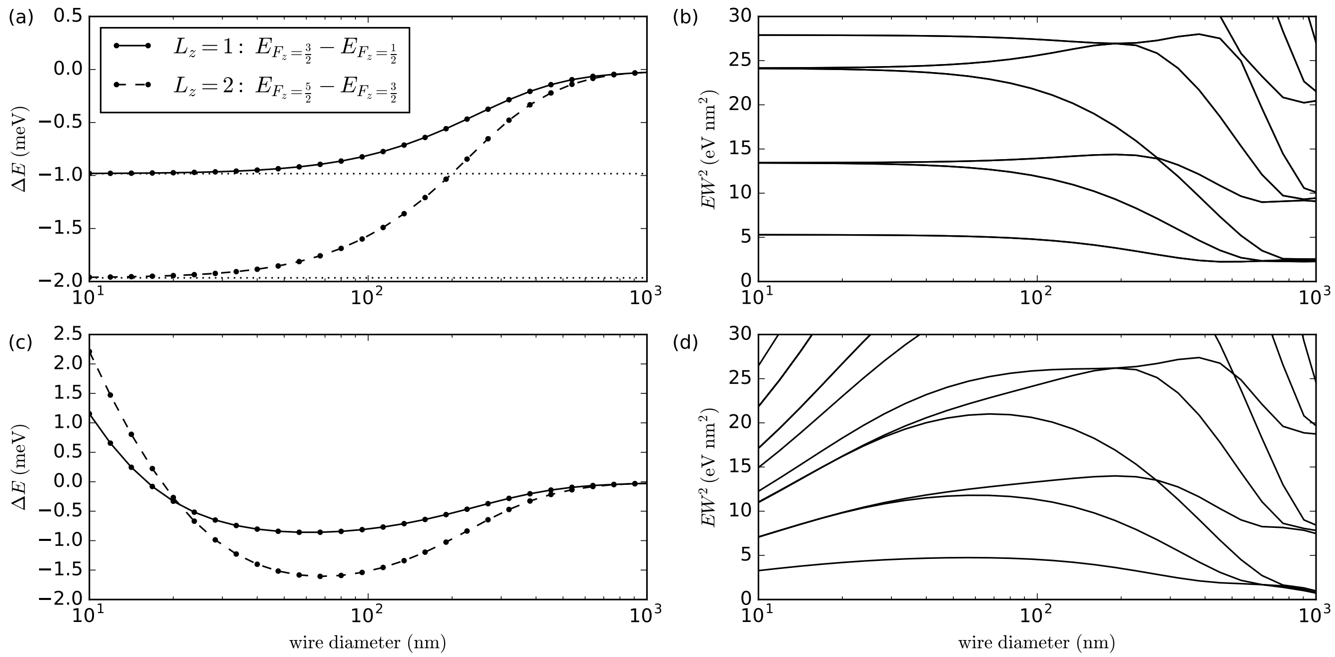


FIG. S2. (a) SOI splitting in the Rashba model wire as a function of wire diameter. The dotted lines are the analytical result of Eq. (S31). (b) Rescaled energies as a function of wire diameter. (c) ((d)) SOI splitting (rescaled energy levels) in an InAs wire obtained by an 8-band $\mathbf{k}\cdot\mathbf{p}$-model for wurtzite InAs.

where in the last approximation we used the renormalized parameters for InSb [5, 6], note that $W$ is the *radius* of the wire.

In the above calculation we used the linearized expression for $E$ and set $E = 0$ in $a$ and $b$. A more precise result can be obtained for thin wires by numerically solving the third order Eq. (S17) for $E$ with $\chi' = z_{lp}$ (no SOI), substituting it in Eq. (S25) and calculating the energy at the modified $\chi'$ by again using Eq. (S17).

## C. Numerical results for wires with soft boundary conditions

All results shown in the main text refer to the hard boundary condition case, where the wave functions is set to zero at the boundary of the wire. Here we instead apply a step potential, which is set to zero inside the wire and 0.2 eV outside of the wire. This mimics the minimal amplitude boundary condition referred to above.

Most results, like the $g$-factors and the magnitude of $\Delta E_l$, are very similar with soft and hard boundary conditions. The most striking difference is that, for soft boundary conditions, and zero magnetic field, the Kramers pair $\left|\pm|l|, \mp\frac{1}{2}\right\rangle$ is higher in energy than the Kramers pair $\left|\pm|l|, \pm\frac{1}{2}\right\rangle$. Thus $\Delta E_l$ has a negative sign in the soft boundary case.

In Fig. S1 we show the SOI splitting for wires with soft boundary conditions. Apart from the sign, the asymptotic behavior is identical. Especially, the $\frac{1}{W^4}$ dependence for large $W$, as in Eq. (S28), is present in both the soft and hard boundary case. Generally, the agreement of the numerics with the analytic approximation Eq. (S28) is quite good.

## D. Numerical results for wurtzite wires

Here we consider InAs wurtzite wires in the 0001 growth direction, as they have been used in Majorana experiments [10]. The main difference in the conduction band of a wurtzite-type semiconductor to a zincblende one is the linear Rashba-like spin-splitting in directions orthogonal to the 0001 wurtzite direction [11]. Therefore, the SOI splitting has a contribution originating from this linear spin splitting. Apart from the origin of the SOI splitting, the mechanism for the enhancement of $g$-factors in wurtzite wires is equivalent to zincblende wires.

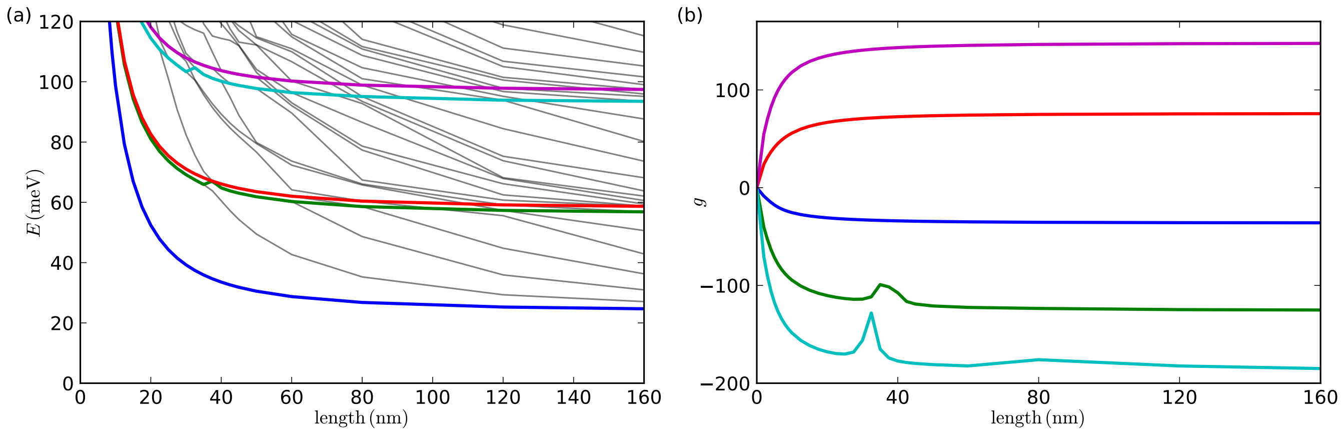


FIG. S3. (a) ((b)) The energy levels ($g$-factors) in a cylindrical InSb quantum dot with 40 nm diameter and variable length. The $g$-factors where evaluated at infinitesimal magnetic field. The lowest five distinct angular momentum subbands are labeled by their color: $l = 0, |f| = \frac{1}{2}$ (blue), $|l| = 1, |f| = \frac{1}{2}$ (green), $|l| = 1, |f| = \frac{3}{2}$ (red), $|l| = 2, |f| = \frac{3}{2}$ (cyan) and $|l| = 2, |f| = \frac{5}{2}$ (magenta). The subbands induced by the confinement in $z$ direction are marked in gray.

We describe the conduction band of wurtzite InAs by a Rashba model

$$H = -\frac{\hbar^2}{2}\left(\frac{k_x^2 + k_y^2}{m_\perp} + \frac{k_z^2}{m_\parallel}\right) + \alpha\left(\sigma_x k_y - \sigma_y k_x\right). \tag{S30}$$

using $m_\perp = 0.0416\, m_e$ and $m_\parallel = 0.0370\, m_e$ [12] and $\alpha = 0.03\,\mathrm{eV\,nm}$ [13]. We solve this model in an infinite wire geometry using cylindrical coordinates as described above. In Fig. S2 (a) we show the SOI splittings $\Delta E_1$ and $\Delta E_2$ as a function of wire diameter. For wire diameters smaller than 100 nm it is approximately constant. For small wire diameters the SOI splitting is approximately given by [14]

$$\Delta E_l = E(l + \frac{1}{2}) - E(l - \frac{1}{2}) = -l\frac{2m^*\alpha^2}{\hbar^2}, \tag{S31}$$

which is in good agreement with our numerical solution. Note that the sign is opposite from the zincblende hard boundary case. For large wire diameters (around 100 nm) the subband splitting becomes of similar size as the SOI splitting leading to a reduction of the SOI splitting. This is also visible in the rescaled energies shown in Fig. S2 (b).

While the Rashba model can explain the origin of the SOI splitting in wurtzite wires it neglects several other aspects like the nonparabolicity of bands and the cubic Dresselhaus splitting. Therefore, we solve the 8-band $\mathbf{k}\cdot\mathbf{p}$-model for wurtzite InAs introduced in Ref. 13 in cylindrical coordinates. Note, that the model is already axially symmetric and no further simplification is needed as in the zincblende case. The results are shown in Fig. S2 (c) and (d). For small wire diameter the cubic in $k$ Dresselhaus spin splitting dominates over the linear in $k$ Rashba splitting and causes an SOI splitting that is different in sign. At large wire diameter the results are very similar to the Rashba model.

### E. Quantum dots

The same reasoning as for wires leads to enhanced $g$-factors in quantum dots with (approximate) cylindrical symmetry. Cylindrically symmetric quantum dots are simulated in the axial approximation. Due to the additional confinement in $z$-direction a 2D boundary value problem needs to be solved now.

In Fig. S3 we investigate the length dependence of the $g$-factor in a short cylindrical InSb wire of 40 nm diameter. The $g$-factors of higher subbands stay larger than the bulk $g$-factor even when the wire length is already much shorter than the wire diameter. The kinks in the $g$-factors result from level crossings with $z$-confinement induced subbands. Therefore, besides wires, the enhanced $g$-factors could be observed in gate-defined quantum dots embedded in a 2DEG, either of circular or approximately square shape (the square case is treated below).

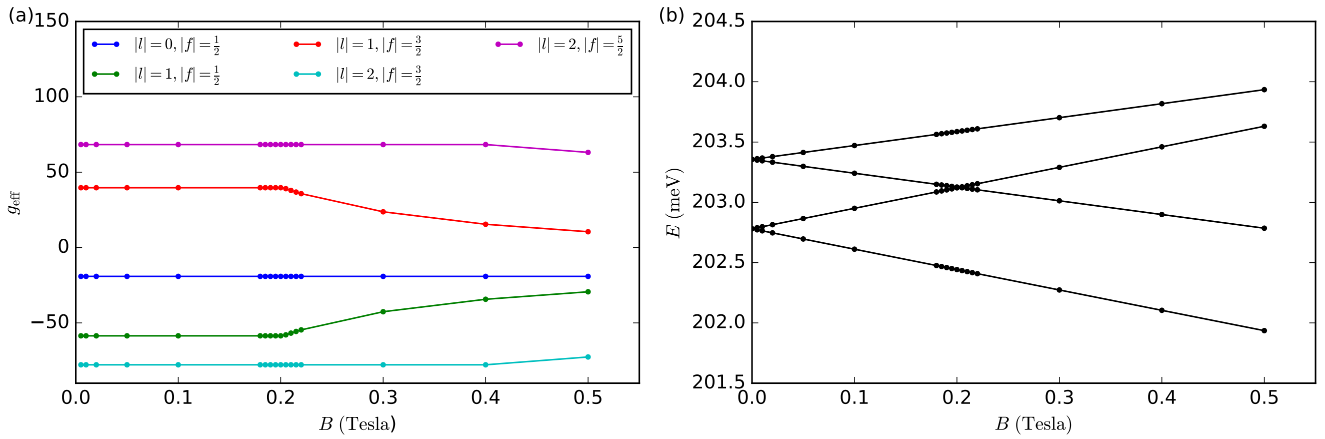


FIG. S4. Tight-binding simulation of a hexagonal InSb wire, grown in the 111 direction, with 20.1 nm diameter. (a) The $g$-factor of the lowest five Kramers pairs in the conduction states as a function of $B$. (b) Energy levels of the lowest $|l| = 1$ states as a function of $B$.

## II. TIGHT-BINDING SIMULATIONS

The $\mathbf{k} \cdot \mathbf{p}$ approximation is only guaranteed to work for long wavelengths and the zincblende $\mathbf{k} \cdot \mathbf{p}$ model used in our simulations neglects the Dresselhaus term, which results from inversion symmetry breaking. For comparison, we also simulate semiconductor wires in zincblende structure using highly accurate first-principles derived tight-binding models. In the tight-binding framework the states are described correctly in the whole Brillouin zone of the lattice, thus, abrupt changes like a hard boundary pose no problem.

For the first-principles calculations we used the Vienna *ab initio* simulation package (VASP) [15, 16] with the projector augmented-wave method, a cut-off energy of 300 eV and using the HSE06 hybrid functional [17–19]. The BZ integration was faciliated with an 8×8×8 Monkhorst-Pack mesh. The effective tight-binding Hamiltonian is generated from the first-principles Wannier functions [20], by projecting the first-principles wave-function on the $s$ and $p$-like orbitals of In, As and Sb. The magnetic field is added via Peierls substitution to the Hamiltonian [21].

In Fig. S4 we show results for a InSb wire grown in the 111 direction and with 20.1 nm diameter. The measured $g$-factors and the critical magnetic field $B_{\rm crit}$ of about 0.2 Tesla agree qualitatively with the $\mathbf{k} \cdot \mathbf{p}$-results presented in the main text. We also find that for the $l \neq 0$ states the Kramers pair with negative $g$-factor, corresponding to $\left|\pm|l|, \mp\frac{1}{2}\right\rangle$, is lower in energy than the one with positive $g$-factor, which corresponds to $\left|\pm|l|, \pm\frac{1}{2}\right\rangle$. Thus, the tight-binding approach gives the same sign of $\Delta E_l$ as the hard wall case in $\mathbf{k} \cdot \mathbf{p}$, justifying our choice of boundary conditions in the main text.

## III. $\mathbf{k} \cdot \mathbf{p}$ SIMULATIONS WITH BROKEN CYLINDRICAL SYMMETRY

### A. Hexagonal wires

In the main text we consider hexagonal wires grown in the 111 direction of a zincblende semiconductor. Again we take the $\mathbf{k} \cdot \mathbf{p}$-parameters from Ref. 4. The 8-band Kane model, this time without the axial approximation, is taken from Ref. 4 and is discretized on a simple cubic lattice. Apart from the Majorana simulations we use a lattice constant of 0.5 nm for the discretization. The wire is built and infinitely extended in the 111 direction. Magnetic and electric fields are added to the lattice Hamiltonian [21]. Note that the simple cubic discretization conserves all symmetries of the cubic zincblende lattice, thus also conserving all symmetries of the wire. Sparse diagonalization is finally used to solve for the eigenenergies and eigenstates of the wire. In Fig. S5 we show results for a hexagonal InSb wire of 40 nm diameter.

In previous 8-band zincblende $\mathbf{k} \cdot \mathbf{p}$ simulations we neglected the Dresselhaus term. While we implicitly checked that the Dresselhaus term does not introduce significant changes via the tight-binding calculation, it is convenient to have a direct comparison of 8-band $\mathbf{k} \cdot \mathbf{p}$ results with and without Dresselhaus term. The Dresselhaus term is added to the 8-band $\mathbf{k} \cdot \mathbf{p}$ Hamiltonian using the definitions and parameters of Ref. 4. In principle, the Dresselhaus term

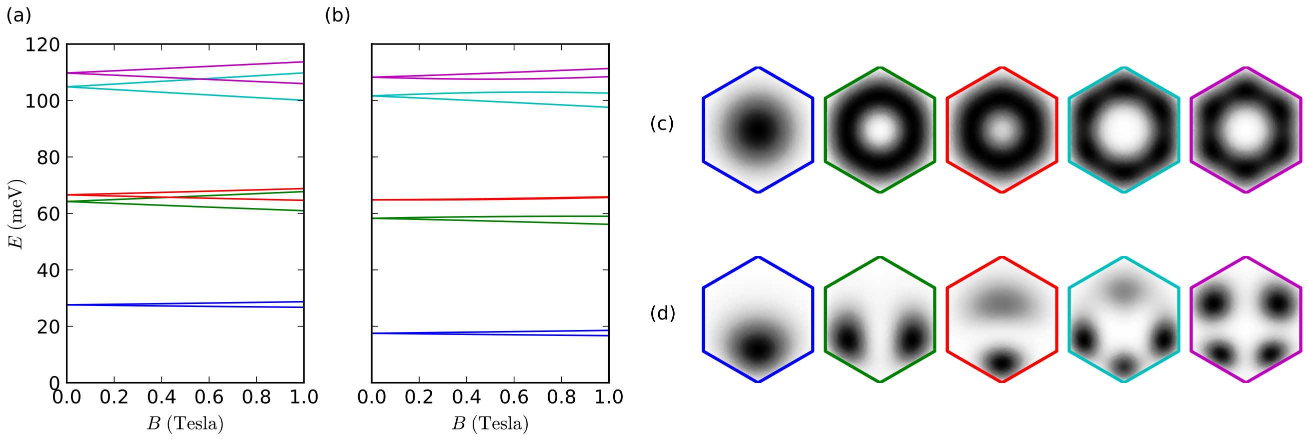


FIG. S5. Hexagonal InSb wire with 40 nm diameter with perpendicular electric field. (a) ((b)) Energy levels of the first ten states as a function of $B$ at an electric field of $\mathcal{E} = 0\,\mathrm{meV/nm}$ ($\mathcal{E} = 3\,\mathrm{meV/nm}$). In the $\mathcal{E} = 0$ case the colors mark different angular momenta. (c) ((d)) Norm squared wave functions of the first five conduction levels at $k = 0$ and $B = 0$ at an electric field of $\mathcal{E} = 0\,\mathrm{meV/nm}$ ($\mathcal{E} = 3\,\mathrm{meV/nm}$).

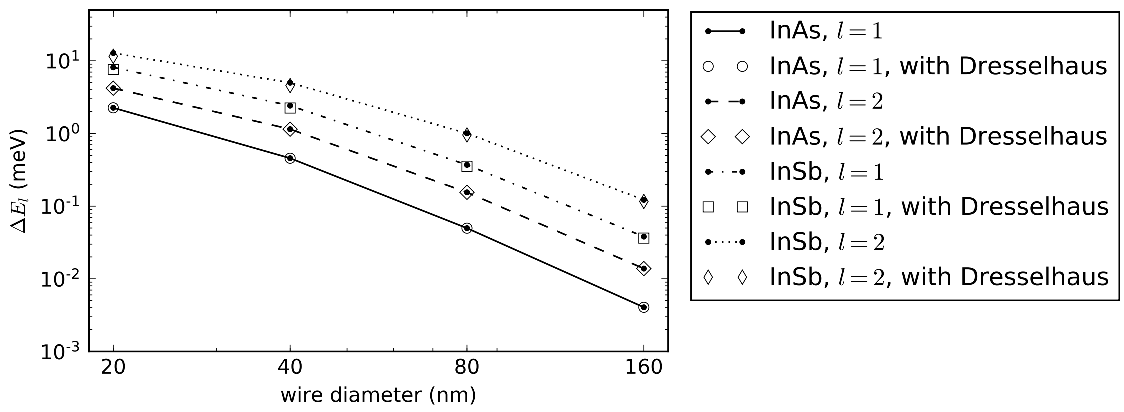


FIG. S6. Diameter dependence of the SOI splitting $\Delta E_1$ and $\Delta E_2$ for hexagonal InSb and InAs wires ($B = 0$ and $\mathcal{E} = 0$). Results with and without Dresselhaus term are compared.

should affect the SOI splitting $\Delta E_l$, like it is the case in wurtzite wires. However, for InAs and InSb it is too small in magnitude to have a significant effect, see Fig. S6.

### B. Rectangular wires

In the main text we focused on hexagonal and cylindrical wires, here we consider now rectangular wires. The parameters of the simulation are identical to the hexagonal case apart from the the growth direction which is now 001.

For a simple quadratic band with effective mass $m^*$ the energy levels at $k = 0$ of a rectangular wire with dimensions $L_x$ and $L_y$ are given by

$$E_{n_x,n_y} = \frac{\hbar^2}{2m^*}\left[\left(\frac{n_x\pi}{L_x}\right)^2 + \left(\frac{n_y\pi}{L_y}\right)^2\right], \tag{S32}$$

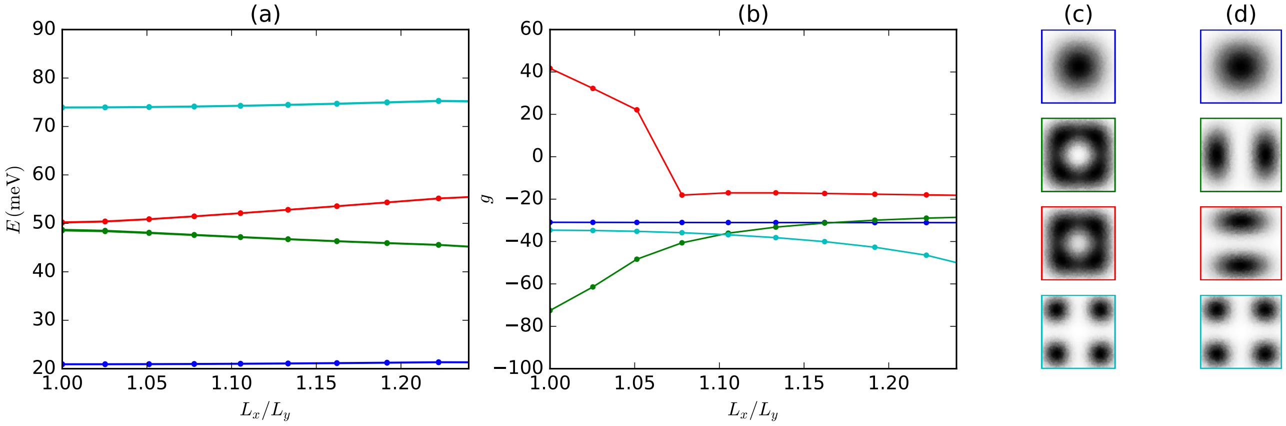


FIG. S7. Results for rectangular InSb wires with fixed crossection of $40 \times 40 = 1600\,\mathrm{nm}^2$ and variable ratio of height to width ($L_x/L_y$). (a) ((b)) Energy levels ($g$-factors) of the first four conduction Kramers pairs as a function $L_x/L_y$. (c) ((d)) Norm squared wave functions of the first four conduction states at $L_x/L_y = 1$ ($L_x/L_y = 1.1$). The color code for the Kramers pairs is the same in (a), (b), (c) and (d).

with the quantum numbers $n_x$ and $n_y$ taking on nonzero positive integer values. The corresponding wavefunctions are given by

$$\psi_{n_x,n_y}(x,y,z) = \frac{1}{\sqrt{N_{n_x,n_y}}} \sin\left(\frac{n_x\pi}{L_x}x\right) \sin\left(\frac{n_y\pi}{L_y}y\right) e^{ikz}, \tag{S33}$$

where $N(n_x, n_y)$ is a normalization factor.

In the case $L_x = L_y$ the lowest energy level is $E_{0,0}$ and the first excited level is two-fold degenerate $E_{1,2} = E_{2,1}$. With SOI the two-fold degeneracy is lifted into two separate states with $f_z \approx \frac{1}{2}$ and $f_z = \frac{3}{2}$ with SOI splitting $\Delta E_1$. Note that due to the $C_4$ symmetry of the wire the angular momenta $f_z = \{-\frac{3}{2}, -\frac{1}{2}, \ \frac{1}{2}, \ \frac{3}{2}\}$ are still in different symmetry sectors. Therefore, we can still talk of the $l \approx 1$ subbands as in the cylindrical case and also the enhanced $g$-factors are found.

This is illustrated in Fig. S7 where a rectangular InSb wire is simulated. For $L_x = L_y$ we find $\Delta E_1$ and the $g$-factor for the $l \approx 1$ bands similar to the cylindrical and hexagonal case. The wavefunctions of the second and third state shown in Fig. S7 (c) are clearly angular momentum eigenstates.

Upon deformation of the quadratic wire the geometry splitting of the second and third state soon surpasses the SOI splitting $\Delta E_1$ and $g$-factors decline rapidly, see Fig. S7 (a) and (b). In the simple quadratic band model the geometry splitting is given by

$$E_{n_x,n_y} - E_{n_y,n_x} = \frac{\hbar^2\pi^2}{2m^*}\left(\frac{1}{L_x^2} - \frac{1}{L_y^2}\right)(n_x^2 - n_y^2), \tag{S34}$$

which is also found in good approximation in our more sophisticated 8-band $\mathbf{k}\cdot\mathbf{p}$ calculation. If $L_x$ and $L_y$ differ enough the geometry splitting exceeds the SOI splitting and the wavefunctions are no more angular momentum eigenstates, see Fig. S7 (d).

### C. Efficient Majorana wire simulations

The realization of Majorana states requires a proximity induced superconducting pairing potential in the wire [22, 23]. For the superconducting calculations we transform the zincblende $\mathbf{k}\cdot\mathbf{p}$ Hamiltonian in the Bogoliubov de Gennes (BdG) basis and double the Hilbert space via adding the hole degrees of freedom. Then, we add an $s$-wave pairing term $\hat{\Delta}$ to the off-diagonal block of the Hamiltonian [24]

$$H_{\mathrm{BdG}}(k_z) = \begin{pmatrix} H(k_z) & \hat{\Delta} \\ \hat{\Delta}^\dagger & -H^*(-k_z) \end{pmatrix}. \tag{S35}$$

The $s$-wave pairing $\hat{\Delta}$ is assumed to be local and is kept constant throughout the wire. Furthermore, we restrict it to the conduction band $s$-like orbitals (the $|u_1\rangle$ and $|u_2\rangle$ basis states), which dominate near the Fermi level. It is then of the form

$$\hat{\Delta} = \Delta \sum_i \left( c^\dagger_{i\uparrow} c^\dagger_{i\downarrow} + \text{h.c.} \right), \tag{S36}$$

where $c$ and $c^\dagger$ are annihilation and creation operators and with $i$ running over all sites and the $s$-like $|u_1\rangle = i\uparrow$ and $|u_2\rangle = i\downarrow$ basis states.

Differential conductivity measurements in semiconductor nanowires in contact to a superconductor are an important probe of possible Majorana states [10, 25–28]. Simulating a realistic infinite wire is already computationally demanding, however, simulating a finite 3D wire long enough to host protected Majorana modes by exact diagonalization would be a hopeless endeavor using current computer hardware. Using the clever Sancho-Rubio scheme [29, 30] it is possible to significantly lessen the computational strain to something which is tractable on modern supercomputers. With the Sancho-Rubio scheme one can simulate the boundary and bulk Greens function of a wire in an iterative fashion, doubling the effective wire length in each iteration [31].

We begin by writing the 1D Hamiltonian in a form that has only nearest neighbor interactions and is translationally invariant inside the wire

$$H_{\text{wire}} = \begin{pmatrix} \epsilon & \alpha & & \\ \beta & \epsilon & \alpha & \\ & \beta & \epsilon & \ddots \\ & & \ddots & \ddots \end{pmatrix}, \tag{S37}$$

where $\beta = \alpha^\dagger$. Longer range interactions can be incorporated by artificially increasing the size of the unit cell such that the effective interactions become nearest neighbor again. Now one can make use of Dyson's identity to write the Green's function $G_{n=2}$ at the left site for a chain of length 2

$$G^{-1}_{n=2} = \omega - \underbrace{(\epsilon + \alpha(\omega - \epsilon)^{-1}\beta)}_{\epsilon^s_1}, \tag{S38}$$

where $\omega$ is the energy and $\epsilon^s_1$ is an effective Hamiltonian for the left surface site. Equivalently, one can attach two sites to the left and to the right to obtain the effective bulk Hamiltonian in the middle of a chain of three sites

$$\epsilon_1 = \epsilon_0 + \alpha(\omega - \epsilon)^{-1}\beta) + \beta(\omega - \epsilon)^{-1}\alpha. \tag{S39}$$

It can be shown that the new effective interactions $\alpha_1$ and $\beta_1$ for the effective Hamiltonians $\epsilon_1$ and $\epsilon^s_1$ are given by [30]

$$\alpha_1 = \alpha(\omega - \epsilon)^{-1}\alpha \tag{S40}$$
$$\beta_1 = \beta(\omega - \epsilon)^{-1}\beta. \tag{S41}$$

Thus the effective Hamiltonian for a system of length $2^l a$, with $a$ being the lattice constant of the chain, can be obtained by iterating the following set of equations

$$\alpha_l = \alpha_{l-1}(\omega - \epsilon_{l-1})^{-1}\alpha_{l-1} \tag{S42}$$
$$\beta_l = \beta_{l-1}(\omega - \epsilon_{l-1})^{-1}\beta_{l-1} \tag{S43}$$
$$\epsilon_l = \epsilon_{l-1} + \alpha_{l-1}(\omega - \epsilon_{l-1})^{-1}\beta_{l-1} + \beta_{l-1}(\omega - \epsilon_{l-1})^{-1}\alpha_{l-1}) \tag{S44}$$
$$\epsilon^s_l = \epsilon^s_{l-1} + \alpha_{l-1}(\omega - \epsilon_{l-1})^{-1}\beta_{l-1}. \tag{S45}$$

The bulk and surface Green's function are given by $G_b = (\omega - \epsilon_l)^{-1}$ and $G_s = (\omega - \epsilon_s)^{-1}$. In practice a small imaginary part is added to $\omega$ to broaden the energy levels for better visibility.

From the diagonal part of the Greens function we obtain the local density of states (LDOS) at the boundary of the wire, which is closely related to the differential conductivity [32]. Due to the increased computational effort a coarser discretization with a lattice constant of 2.5 nm is used in these simulations.

## IV. COMPUTER CODES

We provide the computer code for our $\mathbf{k} \cdot \mathbf{p}$ simulations as supplementary files. All numerical simulations use the Python 3 programming language [33]. Demonstrations of the code are given in form of Jupyter notebooks [34]. The provided `environment.yml` file can be used to create a virtual environment suitable for executing the scripts [35]. Some simulations use the kwant package [36].

- A demonstration of the simulations of the cylindrical zincblende wire with hard and soft boundaries, and also of the finite wire, using the axial approximation is given in `axial_approximation.ipynb`.
- A demonstration of the Rashba model is given in `Rashba_model_cylindrical.ipynb` (and `Rashba_model_dresselhaus.ipynb` with added Dresselhaus term) and a demonstration of the InAs wurtzite wire in `wurtzite_wire.ipynb`.
- A demonstration of the hexagonal zincblende wire is given in `hexagonal_wire.ipynb` and of the rectangular wire in `rectangular_wire.ipynb`.
- The superconducting Hamiltonian is demonstrated in `superconducting_wire.ipynb`. Due to the computational complexity it is recommended to run the 3d Majorana wire simulations on a computing cluster. We provide the python script `calculate_LDOS.py` and sample submit scripts to generate the data for Fig. 5 of the main text.

---


[1] K. J. Vahala and P. C. Sercel, Phys. Rev. Lett. **65**, 239 (1990).
[2] E. Kane, Journal of Physics and Chemistry of Solids **1**, 249 (1957).
[3] P. C. Sercel and K. J. Vahala, Physical Review B **42**, 3690 (1990).
[4] R. Winkler, S. Papadakis, E. De Poortere, and M. Shayegan, *Spin-Orbit Coupling in Two-Dimensional Electron and Hole Systems*, Vol. 41 (Springer, 2003).
[5] F. Nichele, M. Kjaergaard, H. J. Suominen, R. Skolasinski, M. Wimmer, B.-M. Nguyen, A. A. Kiselev, W. Yi, M. Sokolich, M. J. Manfra, F. Qu, A. J. A. Beukman, L. P. Kouwenhoven, and C. M. Marcus, Phys. Rev. Lett. **118**, 016801 (2017).
[6] B. A. Foreman, Phys. Rev. B **56**, R12748 (1997).
[7] L. C. L. Y. Voon, C. Galeriu, B. Lassen, M. Willatzen, and R. Melnik, Applied Physics Letters **87**, 041906 (2005).
[8] S. Çakmak, A. Babayev, E. Artunç, A. Kökçe, and S. Çakmaktepe, Physica E: Low-dimensional Systems and Nanostructures **18**, 365 (2003).
[9] This follows from the identity $\frac{l^2-x^2}{x} J_l(x) = J_l'(x) + x J_l''(x)$.
[10] S. M. Albrecht, A. P. Higginbotham, M. Madsen, F. Kuemmeth, T. S. Jespersen, J. Nygård, P. Krogstrup, and C. M. Marcus, Nature **531**, 206 (2016).
[11] L. C. Lew Yan Voon, M. Willatzen, M. Cardona, and N. E. Christensen, Phys. Rev. B **53**, 10703 (1996).
[12] M. Gmitra and J. Fabian, Phys. Rev. B **94**, 165202 (2016).
[13] P. E. Faria Junior, T. Campos, C. M. O. Bastos, M. Gmitra, J. Fabian, and G. M. Sipahi, Phys. Rev. B **93**, 235204 (2016).
[14] E. N. Bulgakov and A. F. Sadreev, Journal of Experimental and Theoretical Physics Letters **73**, 505 (2001).
[15] G. Kresse and J. Furthmüller, Phys. Rev. B **54**, 11169 (1996).
[16] G. Kresse and J. Furthmüller, Computational Materials Science **6**, 15 (1996).
[17] Y.-S. Kim, K. Hummer, and G. Kresse, Phys. Rev. B **80**, 035203 (2009).
[18] J. Heyd, G. E. Scuseria, and M. Ernzerhof, The Journal of Chemical Physics **118**, 8207 (2003).
[19] J. Heyd and G. E. Scuseria, The Journal of Chemical Physics **121**, 1187 (2004).
[20] A. A. Mostofi, J. R. Yates, G. Pizzi, Y.-S. Lee, I. Souza, D. Vanderbilt, and N. Marzari, Computer Physics Communications **185**, 2309 (2014).
[21] M. Graf and P. Vogl, Phys. Rev. B **51**, 4940 (1995).
[22] R. M. Lutchyn, J. D. Sau, and S. Das Sarma, Phys. Rev. Lett. **105**, 077001 (2010).
[23] Y. Oreg, G. Refael, and F. von Oppen, Phys. Rev. Lett. **105**, 177002 (2010).
[24] M. Tinkham, *Introduction to Superconductivity*, Dover Books on Physics Series (Dover Publications, 1996).
[25] A. Das, Y. Ronen, Y. Most, Y. Oreg, M. Heiblum, and H. Shtrikman, Nat Phys **8**, 887 (2012).
[26] M. T. Deng, C. L. Yu, G. Y. Huang, M. Larsson, P. Caroff, and H. Q. Xu, Nano Letters **12**, 6414 (2012).
[27] V. Mourik, K. Zuo, S. M. Frolov, S. R. Plissard, E. P. A. M. Bakkers, and L. P. Kouwenhoven, Science **336**, 1003 (2012).
[28] H. Zhang, Ö. Gül, S. Conesa-Boj, K. Zuo, V. Mourik, F. K. de Vries, J. van Veen, D. J. van Woerkom, M. P. Nowak, M. Wimmer, D. Car, S. Plissard, E. P. A. M. Bakkers, M. Quintero-Pérez, S. Goswami, K. Watanabe, T. Taniguchi, and L. P. Kouwenhoven, ArXiv e-prints (2016), arXiv:1603.04069 [cond-mat.mes-hall].
[29] M. P. L. Sancho, J. M. L. Sancho, and J. Rubio, Journal of Physics F: Metal Physics **14**, 1205 (1984).
[30] M. P. L. Sancho, J. M. L. Sancho, and J. Rubio, Journal of Physics F: Metal Physics **15**, 851 (1985).
[31] M. Luisier, A. Schenk, W. Fichtner, and G. Klimeck, Phys. Rev. B **74**, 205323 (2006).

[32] S. Datta, *Electronic Transport in Mesoscopic Systems*, Cambridge Studies in Semiconductor Physi (Cambridge University Press, 1997).
[33] https://docs.python.org/3.5/index.html.
[34] http://jupyter-notebook.readthedocs.io/en/latest/.
[35] https://conda.io/docs/using/envs.html.
[36] C. W. Groth, M. Wimmer, A. R. Akhmerov, and X. Waintal, New Journal of Physics **16**, 063065 (2014).
